# Supplementary material for: LawBreaker: An Approach for Specifying Traffic Laws and Fuzzing Autonomous Vehicles
Source: arXiv:2208.14656 source file (2022-10-24)
Supplement: Supplementary file 1 [file Appendix_STL_Formulas.tex]

% \section{appendix}
\section{Proof Of the calculation of $\Theta$}
\label{appendix:proof}
% The proof of Proposition~\ref{prop:overall}:
\begin{proof}
  We first list the following axioms that are assumed to be true.
\begin{itemize}
    \item $\pi \vDash \lnot \mu \implies \pi \nvDash \mu$
    \item $\mathrm{if}\ \Phi = x \land y , \pi \vDash \lnot x \implies \pi \nvDash \Phi, \pi \vDash \lnot y  \implies \pi \nvDash \Phi$
    \item $\mathrm{if}\ \Phi = x \lor y , \pi \vDash (\lnot x \land \lnot y ) \implies \pi \nvDash \Phi$
    \item $N(\neg \theta_1) = \Theta(\theta_1),  \Theta(\neg \theta_1) = N(\theta_1) $
\end{itemize}

If $\Phi$ is $\mu$, we have $\pi \vDash \lnot \mu \implies \pi \nvDash \mu$, so $\Theta(\mu) = \{\neg \mu\}$ is reasonable.

If $\Phi$ is $x \land y $, we have $\pi \vDash \lnot x \implies \pi \nvDash \Phi, \pi \vDash \lnot y  \implies \pi \nvDash \Phi$, so $ \Theta(x \land y ) =  \Theta(x) \cup \Theta(y)$ is reasonable.

If $\Phi$ is $x \lor y $, we have $\pi \vDash (\lnot x \land \lnot y ) \implies \pi \nvDash \Phi$, so $\Theta(x \lor y )= \{x \land y ~|~ x\in \Theta(a) \land y \in \Theta(b)\}$ is reasonable.

If $\Phi$ is $\bigcirc x$, we have $(\pi,t)  \vDash  \bigcirc \Phi \iff (\pi,t+1) \vDash \Phi$. Given $\pi \vDash \lnot \mu \implies \pi \nvDash \mu$, we can get $(\pi,t)  \vDash  \bigcirc \lnot \Phi \iff (\pi,t+1) \nvDash \Phi$.
Hence, $\Theta(\bigcirc x) =  \{\bigcirc x' ~|~ x' \in \Theta(x) \}$ is reasonable.

If $\Phi$ is $x\ \mathcal{U_I} \ y$, in our definition, there are two parts of $\Theta(x\ \mathcal{U_I} \ y)$. The first part is set $\Theta_1$: $\{x' \land y' ~|~ x' \in \Theta(x) \land y' \in \Theta(y)\}$ which implies these equations are satisfies: $\pi \vDash x' \implies \pi \nvDash x, \pi \vDash y' \implies \pi \nvDash y$. Given the definition of $\mathcal{U_I}$: $(\pi,t)  \vDash  x \;\mathcal{U_I}\; y  \iff  \exists t' \in t+\mathcal{I} \text{ such that } (\pi,t') \vDash y \land \forall t'' \in [t,t'], (x,t'') \vDash x $, we can easily get:
\[\forall \xi \in \Theta_1.~\pi \vDash \xi \implies \pi \nvDash x \ \mathcal{U_I}\ y \]
The second part is set $\Theta_2$: $ \{x'~\mathcal{U_I}~y' ~|~ x' \in \Theta(\lnot x \lor y) \land y' \in \Theta(x \lor y)\} $. In order to obtain a contradiction, assume that there is an element $\xi$ of set $\Theta_2$ that satisfies $\pi \vDash \xi \implies \pi \vDash \Phi$. 
Then, 
for $\pi \vDash \Phi$, we get $\exists t' \in t+\mathcal{I} \text{ such that } (\pi,t') \vDash y \land \forall t'' \in [t,t'], (x,t'') \vDash x$, 
which means $(x \land \lnot y)$ is satisfied until $y$ is satisfied. 
For $\pi \vDash \xi$, we get $\exists t' \in t+\mathcal{I} \text{ such that } (\pi,t') \vDash (\lnot x \land \lnot y) \land \forall t'' \in [t,t'], (x,t'') \vDash ( x \land \lnot y)$,
which means $(x \land \lnot y)$ is satisfied until $(\lnot x \land \lnot y)$ is satisfied. 
Hence, at time step $t$, if $x$ is satisfied in $[t,t']$ and violated at time step $t''$ after $t'$, we should get that $y$ is satisfied before $t''$ and $y$ is violated before $t''$ at the same time. This is a contradiction, and so the assumption that there is an element $\xi$ of set $\Theta_2$ satisfies $\pi \vDash \xi \implies \pi \vDash \Phi$ must be false. We can get:
\[\forall \xi \in \Theta_2.~\pi \vDash \xi \implies \pi \nvDash x \ \mathcal{U_I}\ y \] 
Hence,
$\Theta(x\ \mathcal{U_I}\ y) =  \{x'~\mathcal{U_I}~y' ~|~ x' \in \Theta(\lnot x\lor y) \land y' \in \Theta(x \lor y)\} 
 \cup \{x' \land y' ~|~ x' \in \Theta(x) \land y' \in \Theta(y)\}$ is reasonable.

Since the temporal operators $\mathcal{U_I}$ and $\bigcirc$ are
functionally complete, we omit the proof of the remaining temporal operators.
\end{proof}

\section{Implementation}
\label{appendix:Implementation}
We implemented \coolname based on the LGSVL simulation framework and evaluate it with two versions of Baidu Apollo.
Note that our approach can also be implemented for other platforms (e.g.~Carla+Autoware, LGSVL+Autoware) since our specification language and fuzzing algorithms are independent of the underlying simulation environment. The input consists of the scenario description in AVUnit and traffic law specifications in \coolname, whereas the output consists of a set of test cases that violate those traffic laws in different ways.
In the following, we briefly describe the various modules we implemented to connect the specification parser, the fuzzing engine, and the simulator with ADS frameworks. The source code is available at~\cite{ourweb}. 
% \todo{Make sure to provide a link to the source code on the website. SY:Added already}

In the parser module, the script is divided into two parts: the scenario description and the traffic laws.
These two parts are parsed separately since the traffic laws can be translated to an independent abstract syntax tree~(AST) for the simulator, i.e.~without the scenario constructs.
Our parser for \coolname is implemented using \emph{ANTLR4}~\cite{antlr4}.
The parser checks the grammar of the specifications and translates our language to standard STL formulas. 

Since customisation is necessary for the simulators and ADSs, we need a bridge that adapts the scenarios to a format recognised by the simulator, and also collects and
extracts the variables that we describe in Section~\ref{sec:Spec} from the messages published by the ADS.
% parses the messages published by the ADS into the signal variables we described in Section~\ref{sec:Spec}.
Hence, the bridge can spawn scenarios for the simulator and generate a trace using the collected data.

Our detailed fuzzing algorithm was described in Section~\ref{sec:Fuzzing}. Our implementation supports the mutation of six categories, i.e.~position, speed, time, weather, NPC vehicle type, and pedestrian type. 
Furthermore, we embedded the tool \emph{RTAMT}~\cite{nivckovic2020rtamt} to compute the robustness of the specifications with respect to the trace obtained from the bridge. 

The maps we use are all from the map store~\cite{lgsvl_maps} of LGSVL. For the Car model, we choose \emph{LincolnMKZ2017}---the detailed model information can be found online~\cite{lgsvl_vehicles}. The available sensor modules (e.g.~Planning, Control, Prediction, PerceptionObstacle) of Apollo are all enabled to ensure that the ADS can run normally. Note that since our goal is to test the ADS and the perception part of Apollo~6.0 is still under development, we follow the recommendation of the vendor and use ground truth as the input.% of the module $\mathtt{PerceptionObstacle}$.
